# Supplementary material for: Vision-centric Token Compression in Large Language Model
Source: arXiv:2502.00791 source file (2025-12-11)
Supplement: Supplementary file 1 [file appendix_more_methods.tex]

\begin{table}[t]
\caption{\textbf{Comparison with vision-centric and Long-context models.} on In-context Learning (SST5 and DBP) and Open-domain QA (TriviaQA, NQ, and PopQA) tasks. 
}
\label{table:appendix:more_methods}
\begin{center}
\begin{small}
% \renewcommand\arraystretch{1.1}
% \resizebox{0.8\textwidth}{!}{
\begin{tabular}{lcccccccccc}
            \toprule
           \textbf{Method} & $n_\text{e}$ & $n_\text{d}$ & \textbf{SST5} & \textbf{DBP} & $k_\text{e}$ &$k_\text{d}$  & \textbf{TriviaQA} & \textbf{NQ} & \textbf{PopQA} \\
            \midrule

            Replug & - & 20 & 29.1& 7.3&  - & 15 &16.07 &6.32 & 4.77\\

            Stream & - & 20 & 29.7& 70.5&  - & 15 &15.13& 7.11& 5.12\\
        
            ToMe$^{\dagger}$  & 18 & 2 &22.0 & 68.0 & 5 & 10&14.37 &6.92 & 4.13\\

            FastV$^{\dagger}$ & 18 & 2
 &24.8 &65.4& 5 & 10 &14.69 &6.08 & 4.96\\

            \ourname & 18 & 2 & \bf42.7 & \bf71.9  & 5 & 10 &\bf25.20&	\bf8.71	&\bf11.44  \\

            \bottomrule
        \end{tabular}
% }

\end{small}
\end{center}
\end{table}
